# Supplementary material for: Asymptotic Cellular Growth Rate as the Effective Information Utilization Rate
Source: arXiv:1308.0623 source file (2014-03-12)
Supplement: Supplementary file 1 [file suppMattEndGameResub6.pdf]

# "Asymptotic Cellular Growth Rate as the Effective Information Utilization Rate" - Supplementary Material

Rami Pugatch, Naama Barkai and Tsvi Tlusty


## abstract

In section (I) of the supplementary material we derive (a) the optimal utilization strategy for a given information channel (characterized by its distribution of side-information conditioned on the environment), (b) the optimal bet hedging strategy given the distribution of environment and (c) the min-max optimal solution. In section (II) we present the results of a Monte-Carlo simulation of the experiment suggested in the paper, which validates our main result in a particular case. In section (III) we demonstrate how one may employ our formalism to study bacteria in batch, where growth is non-exponential. In section (IV) we present a derivation of the optimal switching strategy when the environment distribution is not stationary. In section (V) we present two possible experiments and discuss the interesting form of the of the non-diagonal growth matrices related to them. In section (VI) we present a code for reducing any growth matrix to its essential part that also solves for the game-theoretic optimum.


## (I) Derivation of the optimal utilization strategy

We derive the optimal utilization strategy given the information channel performance characterized by the distribution of its output given the external environment. Our starting point is the ensemble average asymptotic growth rate derived in the paper:

$$\Lambda = \sum_{ij} p_{ij} \log\left(\sum_{k'} O_{ik'} b_{k'|j}\right). \quad \text{(S1)}$$

To find the optimal phenotype distribution given the performance of the information channel as characterized by the joint probability distribution $p_{ij}$ ($i$ being the index of the environment and $j$ of the side information about it), we equate to zero the derivative of Eq. (S1) with respect to $b_{k|l}$, using Lagrange multipliers to ensure that we stay within the probability simplex (i.e. that $\sum_k b_{k|j} = 1$, for all $j$ ):

$$\frac{d}{db_{k|l}}\{\Lambda - \sum_j \lambda_j \sum_{k'} (b_{k'|j} - 1)\} = 0,$$

$$\Rightarrow \frac{d}{db_{k|l}}\{\sum_{ij} p_{ij}\log\left(\sum_{k'} O_{ik'}b_{k'|j}\right) - \sum_j \lambda_j \sum_{k'}(b_{k'|j}-1)\} = 0,$$

$$\Rightarrow \sum_{ij} p_{ij}\frac{\sum_{k'} O_{ik'}\delta_{jl}\delta_{k'k}}{\sum_{k'} O_{ik'}b_{k'|j}} - (\sum_j \lambda_j \sum_{k'} \delta_{jl}\delta_{k'k}\} = 0,$$

$$\Rightarrow \sum_i p_{il}\frac{O_{ik}}{\sum_{k'} O_{ik'}b_{k'|l}} = \lambda_l.$$

Define now $y_{i|l} \triangleq \sum_{k'} O_{ik'}b_{k'|l} > 0$ and define $z_{i|l} \triangleq \frac{p_{il}}{y_{i|l}}$

Then we have

$$\sum_i p_{il}\frac{O_{ik}}{y_{i|l}} = \lambda_l \Rightarrow \sum_i O_{ik}\, z_{i|l} = \lambda_l,$$

or in matrix form

$$O^t|z_{\cdot|l}\rangle = \lambda_l|1\rangle,$$

where the $|z_{\cdot|l}\rangle$ is a column vector with the $i^{th}$ element equal to $z_{i|l}$, $O^t$ is the transpose of O and $|1\rangle$ is the all-one column vector.

We can solve this equation assuming $O^t$ is invertible from the left, but for simplicity we will assume it is square and invertible (the meaning of this assumption is that we focus on the essential part of the game as explained in the paper). Then we have:

$$|z_{\cdot|l}\rangle = \lambda_l(O^t)^{-1}|1\rangle.$$

Now let us write this equation again in coordinates (remembering that $(O^t)^{-1}=(O^{-1})^t$ and substituting the definition of $z_{i|k}$) to obtain:

$$\frac{p_{il}}{y_{i|l}} = \lambda_l\sum_j (O^{-1})_{ji} \;\Rightarrow\; \frac{p_{il}}{\sum_j (O^{-1})_{ji}} = \lambda_l y_{i|l}$$

Substituting the definition of $y_{i|l}$ we obtain:

$$\frac{p_{il}}{\sum_j (O^{-1})_{ji}} = \lambda_l \sum_{j'} O_{ij'}b_{j'|l} \qquad \text{(S2)}$$

we define the diagonal matrix d such that

$$d_{ij} = \frac{\delta_{ij}}{\sum_k (O^{-1})_{ki}}$$

Where $\delta_{ij}$ is the Kronecker delta ($\delta_{ii} = 1$, $\delta_{ij} = 0, i \neq j$). In words: the *k*-th element in the diagonal of d is the reciprocal of the sum of the columns of the *k*-th row of the matrix $O^{-1}$.

Then we can write Eq. (S2) in matrix form as

$$d|p_{\cdot,l}\rangle = \lambda_l O|b_{\cdot|l}\rangle, \qquad \text{(S3)}$$

where $|p_{\cdot,l}\rangle$ is a column vector with the i[th] element being equal to $p_{il}$ and $|b_{\cdot|l}\rangle$ is also a column vector with the i[th] element being equal to $b_{i|l}$. Multiplying Eq. (S3) by $O^{-1}$ on both sides we obtain:

$$|b_{\cdot|l}^{opt} >= \lambda_l^{-1} W\ |p_{\cdot,l} >, \qquad \text{(S4)}$$

where W is defined as:

$$W \triangleq O^{-1}D \qquad \text{(S5)}$$

Alternatively, in coordinates,

$$W_{ij} \triangleq \sum_k O_{ik}^{-1} \frac{\delta_{kj}}{\sum_{k'} O_{k'j}^{-1}} = \frac{O_{ij}^{-1}}{\sum_{k'} O_{k'j}^{-1}}$$

Then the optimum solution (Eq. (S4)) in coordinates is given by:

$$b_{i|l}^{opt} = \frac{\sum_j W_{ij} p_{jl}}{\sum_{ij} W_{ij} p_{jl}}, \qquad \text{(S6)}$$

where we used the normalization condition $\sum_k b_k = 1$ which yields $\lambda_l = \sum_{ij} W_{ij} p_{jl}$.

We simplify Eq. (S6) further by noting that

$$\sum_i W_{ij} = \sum_i \frac{O_{ij}^{-1}}{\sum_{k'} O_{k'j}^{-1}} = 1$$

It follows that $\lambda_l = p_l \triangleq \sum_j p_{jl}$. Inserting to Eq. (S6) and using $p_{jl} = p_{j|l} p_l$ we obtain that

$$b_{i|l}^{opt} = \sum_j W_{ij} p_{j|l}\ , \qquad \text{(S7)}$$

which is the result used in the paper. We note that $W^{-1} = D^{-1}O$ thus

$$W_{ij}^{-1} = \sum_k \sum_l O_{li}^{-1}\, \delta_{ik} O_{kj} = \sum_l O_{li}^{-1}\, O_{ij}$$

Clearly,

$$\sum_i W_{ij}^{-1} = \sum_{il} O_{li}^{-1} O_{ij} = \sum_l \delta_{lj} = 1$$

It follows that a necessary and sufficient condition for $S^{-1}$ to qualify as a stochastic matrix is for the columns of the inverse of the growth-phenotype matrix O to be positive:

$$W^{-1} \text{ stochastic } \Leftrightarrow \sum_i O_{ij}^{-1} > 0. \qquad \text{(S8)}$$

Next we derive the optimal bet-hedging strategy given the distribution of environments. This is a corollary of Eq. (S7) upon removal of the side information with the result

$$b_i^{opt} = \sum_j W_{ij} p_j \qquad \text{(bet-hedging)} \qquad \text{(S9)}$$

Using the optimal bet-hedging strategy we can calculate the game-theoretic solution to the game. For that purpose, we reduce Eq. (S1) for the AGR by eliminating the side information variable to obtain that $\Lambda_{\text{bet}} = \sum_i p_i \log\left(\sum_{j'} O_{ij'} b_j^{opt}(p_i)\right)$. Inserting Eq. (S9) and taking the derivative with respect to *p* using a Lagrange multiplier to keep the variables within the probability simplex we obtain:

$$\frac{d}{dp_j}\{\Lambda_{\text{bet}} - \lambda(\sum_i p_i - 1)\} = 0$$

$$\Rightarrow \frac{d}{dp_j}\{\sum_i p_i \log\left(\sum_{j'} O_{ij'} b_j^{opt}(p_i)\right) - \lambda(\sum_i p_i - 1)\} = 0$$

Inserting $|b^{opt}\rangle = S|p\rangle$ we obtain

$$\Rightarrow \frac{d}{dp_j}\{\sum_i p_i \log\left(\sum_{jj'} O_{ij'} S_{j'j}\, p_j\right) - \lambda(\sum_i p_i - 1)\} = 0$$

Inserting the definition of $S_{ij}$ we obtain

$$\Rightarrow \frac{d}{dp_j}\{\sum_i p_i \log\left(\sum_{jj'} O_{ij'} O_{j'j}^{-1} D_{jj}\, p_j\right) - \lambda(\sum_i p_i - 1)\} = 0$$

This further simplifies to

$$\frac{d}{dp_j}\{\sum_i p_i \log(d_{ii}p_i) - \lambda(\sum_i p_i - 1)\} = 0$$

$$\Rightarrow \sum_i (\delta_{ij}\log(d_{ii}p_i) + \frac{1}{d_{ii}} d_{ii}\delta_{ij}) = \lambda \Rightarrow \log\left(d_{jj}p_j\right) = \lambda - 1$$

$$d_{jj}p_j = e^{\lambda-1} \Rightarrow p_j^* = \frac{d_{jj}^{-1}}{\sum_j d_{jj}^{-1}}, \qquad \text{(S10)}$$

which is the game theoretic optimum. Inserting Eq. (S10) to Eq. (S9) we obtain

$$b_j^* = \sum_j W_{ij} \frac{d_{jj}^{-1}}{\sum_j d_{jj}^{-1}}$$

Or, by inserting the definition of *D* and *S* we obtain that

$$p_j^* = \frac{\sum_k O_{kj}^{-1}}{\sum_{jk} O_{kj}^{-1}}$$

$$b_i^* = \sum_j O_{ij}^{-1} D_{jj} \frac{\sum_k O_{kj}^{-1}}{\sum_{jk} O_{kj}^{-1}} = \sum_j \frac{O_{ij}^{-1}}{\sum_{jk} O_{kj}^{-1}} \ . \qquad \text{(S11)}$$

Finally, the game value is given by Λ(b*,p*)=-$\log_2(\sum_{jk} O_{kj}^{-1})$ upon substitution of Eqs. (S11) to $\Lambda_{\text{bet}}$.

## (II) Monte-Carlo (MC) simulation to verify our results

We performed a MC simulation to test our formula in a particular scenario. We consider a cell growing in a fluctuating environment with two possibilities E=1 or E=2. We assume the cell has an information channel with a performance matrix

$$\Pi = \begin{pmatrix} Pr(s=1, E=1) = 0.85 & Pr(s=2, E=1) = 0.1 \\ Pr(s=1, E=2) = 0.15 & Pr(s=2, E=2) = 0.9 \end{pmatrix},$$

the growth matrix that is given by

$$O = \begin{pmatrix} Pr(E=1, B=1) = 1.13 & Pr(E=1, B=2) = 1.05 \\ Pr(E=2, B=1) = 0.89 & Pr(E=2, B=2) = 1.05 \end{pmatrix},$$

(numbers are chosen to fit known data on e-coli growth assuming dwell time of 3 hours).

Finally, the utilization matrix is given by

$$B = \begin{pmatrix} Pr(\varphi=1, S=1) = 0.8 & Pr(\varphi=2, S=2) = 0.1 \\ Pr(\varphi=1, S=2) = 0.2 & Pr(\varphi=2, S=2) = 0.9 \end{pmatrix}.$$

We varied the probability for environment E=1 (Pr(E=1)), creating for each value a long sequence of 250000 random samples with this distribution, and calculating the AGR either directly from its definition or using our formula.

More specifically, the algorithm consists of the following steps (code available upon request)

1. Generate a random sequence of environments with probability **p**.
2. Run over the random sequence of environments and choose for each cell the side information and the phenotype given the side information assuming all cells share the same distributions for the channel performance and phenotypic switching response (conditioned on side information).
3. For each phenotype calculate the growth factor per cell.
4. Calculate the time averaged AGR.
5. Calculate the information utilization rate U.
6. Repeat for M times and average to obtain a direct estimate of the AGR, compare with the sum: D( p || p* ) + U + $\Lambda_{game}$.
7. Plot the results of the MC simulation vs. our prediction for several different strategies.

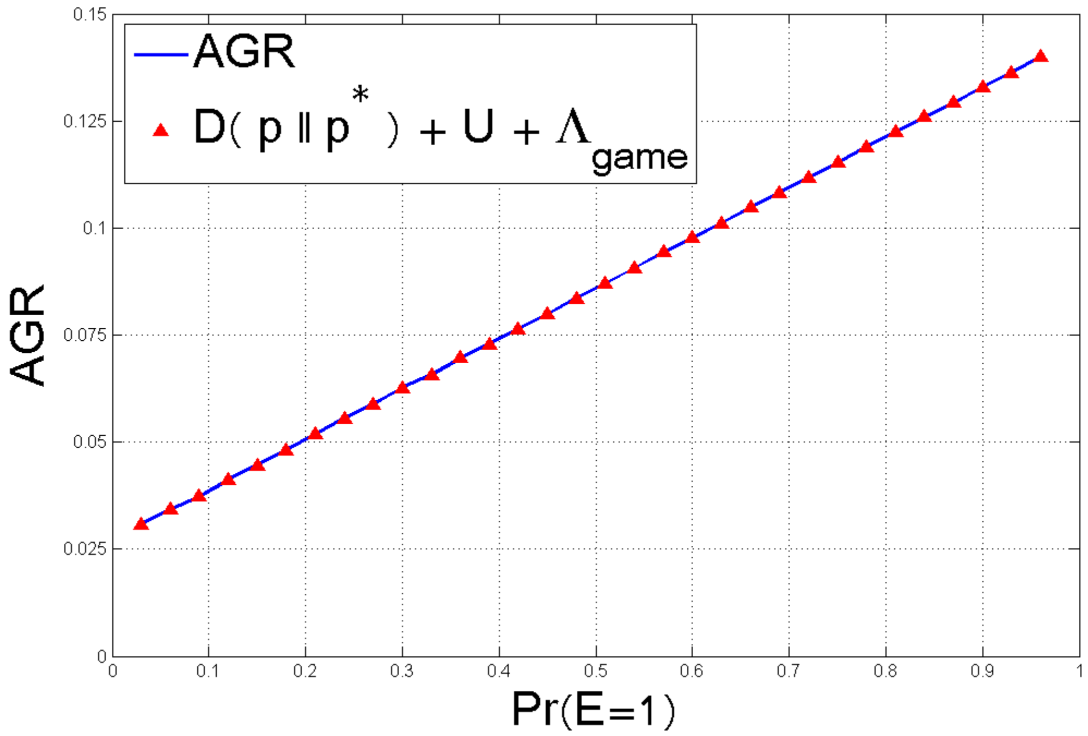


Fig. S1: Validation of the asymptotic growth rate formula in the binary environment scenario described in the text. Number of MC runs was 250000. Blue Line – direct calculation of the time-averaged AGR; red line – calculation of the AGR by summing the estimate of D(p||p*) and the information utilization rate U from the data.

## (III) The transporters game

Consider E. coli bacteria growing in a constant environment. Maintaining a constant environment is feasible by either actively stabilizing the environment or constantly replenishing the media while keeping the cells in small quantities such that their effect on the environment is negligible. For a recent implementation of such a system see [A1].

Let the environment be characterized by a list of concentration vectors $\vec{c} = (c_1, c_2, \dots, c_n)$. We only consider chemically defined media, where the vector $\vec{c}$ is well defined (both in term of preparation and measurement). Each concentration is allowed to vary within an interval $c_{i,min} \leq c_i \leq c_{i,max}$, which we discretize to small bins of size $\Delta c_i$. Thus we obtain $n_1$ discrete environments for $c_1$, $n_2$ discrete environments for $c_2$ etc, so the total number of discrete environments is $n_E = \prod_{i=1}^{n} n_i$ which we can order arbitrarily. This defines the set E={1,…,$n_E$}.

Next, we operationally define the side information. For each environment in the list, we find the optimal growth rate. In practice, this implies that a large number of measurements should be taken in each environment, and that the maximum growth rate is recorded. For simplicity, we will assume a single parameter *c* to define this environment (*c* may be temperature or pH or concentration of glucose etc.).

After the measurements we obtain a functional relation of the form

$$\mu_{max} = f(c). \qquad \text{(S12)}$$

Where f(c) is a fitting function found empirically from the measurements (an interesting separate challenge would be to predict *f* ab-initio).

Can we infer how well the cells are informed about the parameter c from a measurement of their actual growth rate? If the environment is fixed and there is a single limiting nutrient c, we answer in the affirmative.

Consider then the case where *c* is the external single carbon source concentration. It was found empirically that if c stands for glucose, the function *f* can be described using three *fitting parameters* $h_i$, $K_i$ and $V^{max}_i$ such that

$$\mu_{max} = \bar{\mu} \frac{c_i^h}{K_i^h + c_i^h} \quad , \qquad \text{(S13)}$$

where $\bar{\mu}$ is the maximal growth rate over all environments (see [A2] and references therein).

The actual growth rate may still be less than this maximum for at least two reasons: (i) the cell might uptake less than the optimal amount of the limiting nutrient; (ii) the yield (change in relative growth per amount of nutrient consumed) might not be optimal. The first case corresponds to a profile of transporters that is not optimal for the environment, while the second refers to the case where the internal machinery is not optimally matched to the actual transport rate.

We define the actual growth rate as

$$\mu = Y_i(c_i^{eff})\bar{\mu}\frac{(c_i^{eff})^h}{K_i^h+(c_i^{eff})^h} \quad , \qquad \text{(S14)}$$

which differs from the maximum $\mu_{max}$, because the effective environment – the environment the cell happens to be optimal for, differs from the current environment. Also, the yield can be smaller than one: $Y_i(c_i^{eff})<1$ (we normalize the yield such that its maximum is one).

For simplicity, we will neglect the effect of the yield by assuming it is always maximal. We interpret the quantity $c_{eff}$ as the sensed concentration or, upon discretization, the *side information*. To be more explicit, by inverting Eq. S14 we find that:

$$c_{eff} = {\mu_{max}}^{-1}(\mu) = K(\frac{x}{1-x})^{\frac{1}{h}},$$

where $= \frac{\mu}{\mu_i^{max}}$. In this case, for any $c_{eff}$ we can find an index $s \in E$, such that $c_s \leq c_{eff} \leq c_s + \Delta c$. So *s* is interpreted naturally as the side-information regarding the concentration c.

The cell has an arsenal of transporters at its disposal from which it can choose a mixture that will determine the overall rate of transport of nutrient c. Since the yield is constant in our example, this also determines the actual growth rate $\mu$. Rewriting S14 we obtain

$$\mu = Y_i(c_i^{eff})\bar{\mu}\varphi_k(c_{eff}|c)=\bar{\mu}\varphi_k(c_{eff}|c),$$

where the second equality stems from our assumption regarding optimal yield. The function $\varphi_k(c_{eff}|c)$ is interpreted as the actual transport rate of *c* by a cell exhibiting phenotype k due to the side information $c_{eff}$.

Each transporter mixture is optimal within certain bounds. To implement this heuristically we use the following function

$$\varphi_k(c_{eff}|c) = \frac{A_k}{\cosh^2(\beta_k(c-c_k))},$$

where $\beta_k$ controls the size of the window where the transporter can function properly, $A_k$ the maximal performance, and $c_k$ is the location of the peak performance, so $c_{eff} = c_k$.

Thus, the actual growth rate, in discrete units is

$$\mu_{e=i,b=k} = \mu_i^{max} \frac{\left(\frac{A_k}{\cosh^2(\beta_k(c-c_k))}\right)^h}{K_i^h + \left(\frac{A_k}{\cosh^2(\beta_k(c-c_k))}\right)^h} . \qquad \text{(S15)}$$

To summarize, the cell decides on its phenotype (=transport type mixture that in turn determines the transport rate) by sensing the environment ($c_{eff}$). It then grows at an effective rate $\mu$. Each phenotype grows at a different rate in a given environment, as described by Eq. S4. We supplement the dynamics by specifying a transition rule that specify how the cells switch between phenotypes as the imperfect side information stochastically changes.

<u>Non-exponential growth curves</u>

If we place a population of cells in a batch culture with an initial concentration of glucose, what will be the dynamics? The cells sense the presence of glucose imperfectly and tune their transporters combination fast (this is our assumption of fast switching). However, as they consume the glucose, the concentration in the external environment changes. As the cells constantly sense the environment and respond they also sense this change, again imperfectly, and adapt their phenotype according to the changes they induced. This feedback goes on continuously until the nutrient is totally depleted from the environment.

Both the information about the environment and the corresponding response to it are not necessarily optimal in our formalism. It follows that the cells do not simply track the environment using the optimal phenotype. Due to the constant feedback between the phenotype and the environment, and the imperfect and stochastic nature of the sensing and utilization of information, the entire path (and in particular the overall population size as a function of time) is stochastic. However, the average response reflects the average information the population process.

The equations of motion of such a dynamical system can be written as follows:

$$\frac{dN_k}{dt} = \mu_{ik} N_k + \sum_{k=1}^{N_B} W_{kj} N_j$$

where $W_{km}(t, t'|c)$ is the transition matrix from phenotype *m* to phenotype *k* given the environment *c(t)*. In the limit where the transition rate is faster than the growth rate, we can rewrite this equation as

$$\frac{dN_k}{dt} = N\mu_{ik} b_{k|s}$$

where $b_{k|s=j}$ is the steady state solution of $W_{km}(t,t^{'}|c(t) = c_i)$ and the side information $s$ is defined by $\lim_{n\to\infty} \operatorname{argmin}(|p - S^{-1}(W)^n \vec{b}\,|)$ i.e. the index of the environment the cell is optimal for with the current phenotype.

The environment is also changing according to the following equation:

$$\frac{dc_i}{dt} = -N\mu_{ik} b_{k|j}$$

<u>Simulation the growth curve dynamics</u>

To simulate the above dynamics we use the following algorithm

1. Update the environment concentration to c(t).
2. All cells sense the glucose. Their transition matrix is W(c). The sensing (information) channel has a performance matrix P $\approx W(c)^n, n \gg 1$.
3. During a short time interval $\delta t$ for which the environment is assumed fixed and equals to $c(t)$, the population grows by a factor $\sum_{k=1}^{N_B} \mu_{ik}\, b_k$.
4. Update the concentration to $c(t+\delta t) = c(t) - \frac{1}{Y_c} N(t) \sum_{k=1}^{N_B} \mu_{ik}\, b_k \delta t$
5. Update current time to t---> t+ $\delta t$.
6. Repeat until depletion (c=0).

<u>Simulation Results</u>

In Figure S1 we show the growth matrix (Eq. S15), and the reduced growth matrix, obtained by eliminating the dominated phenotypes and environments. The number of different transporters (phenotypes) is eight and we assume constant yield.

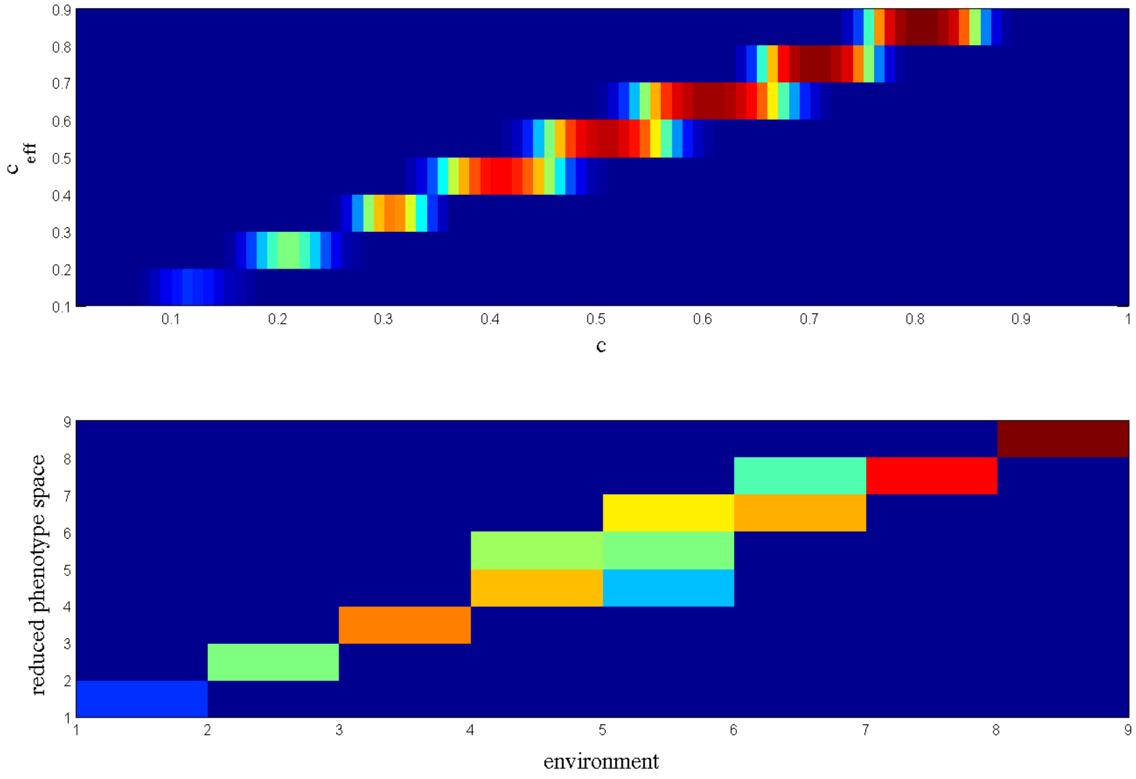


Figure S1. The growth matrix (Eq. S15) (upper image) and its reduced form (lower image), blue represents low growth rates and red represents high growth rates.

Figure S2 shows the resulting non-exponential growth obtained in batch conditions. The transitions between phenotypes (transporter mixtures) are similar to a diauxic shift, as the cells consistently, yet stochastically, drift towards the optimal transporter mixture which has the highest growth rate (given their imperfect information about the environment, and their imperfect utilization of that information).

The transition occurs whenever the environment changes are sufficient to render the current phenotype suboptimal according to the cells state of knowledge. The noisy information channel smoothen the transition which would otherwise be sharp.

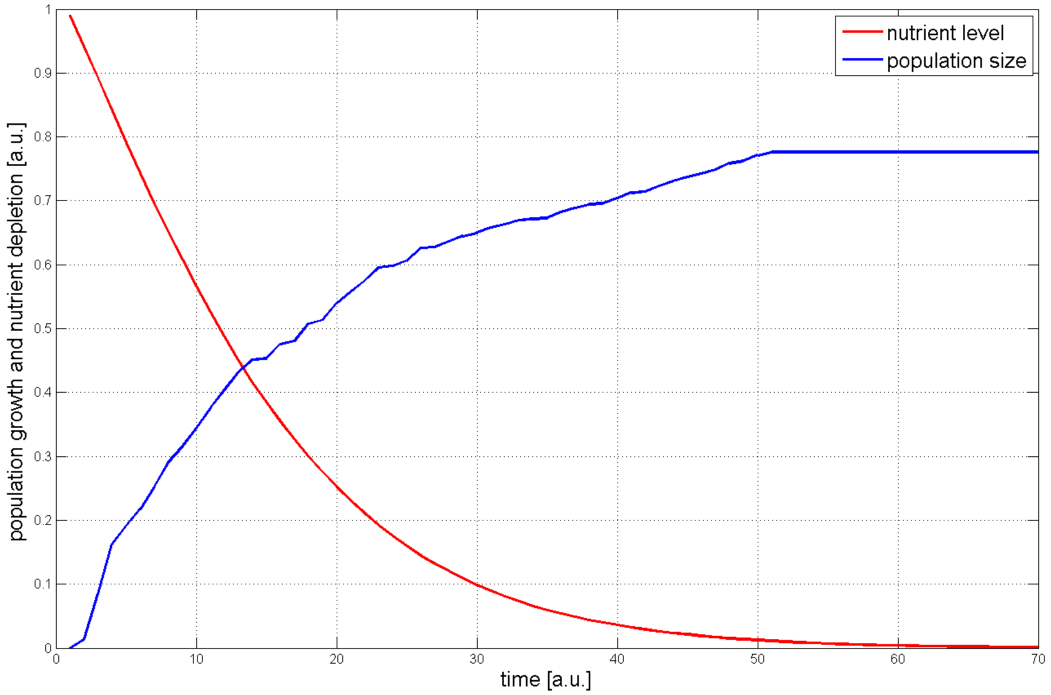


Figure S2: Batch growth simulation with imperfect sensing of the environment. Growth curve is clearly non-exponential due to the continuous consumption of sugar.

An interesting future direction would be to find a method to infer the information utilization rate directly from a growth curve, which is more accessible experimentally compared to the more controlled experiment suggested in the paper.

## (IV) Non-stationary environments – the adiabatic limit

Consider random fluctuating environments with a distribution that is changing with time. Assume that for all times the rate of change is slower compared to the relaxation rate to equilibrium. The instantaneous loss is given by

$$L(t) = \sum_{ij} p_{i|j}(t) p_j^s \log\left(\frac{p_{i|j}(t)}{\sum_k W_{ik}^{-1} b_{k|j}(t)}\right).$$

The best strategy to minimize the loss is to instantaneously tune $b_{k|j}(t)$ however, in practice, this rarely happens since there are both time and cost constraints for phenotype switching.

To proceed without introducing cost explicitly, we assume that there is a time window for doing the adjustment and that this time window from $t_v$ to $t_{v+1}$, allows a single readjustment of strategy $b_{k|j}$. To find the optimal readjustment under this constraint we need to minimize

$$\int_{t_v}^{t_{v+1}} L(t)dt - \lambda\left(\sum_k b_{k|j} - 1\right) = \int_{t_v}^{t_{v+1}} \sum_{ij} p_{i|j}(t) p_j^s \log\left(\frac{p_{i|j}(t)}{\sum_k W_{ik}^{-1} b_{k|j}(t)}\right) dt - \lambda\left(\sum_k b_{k|j} - 1\right).$$

Taking derivative with respect to $b_{k|j}$ and equating to zero we find that

$$\sum_k W_{ik}^{-1} b_{k|j}^{opt} = \frac{1}{t_{v+1} - t_v} \int_{t_v}^{t_{v+1}} p_{i|j}(t)\, dt,$$

Or in vector form $\boldsymbol{b}^{opt} = W\overline{\boldsymbol{p}}$, where $\overline{\boldsymbol{p}} = \frac{1}{t_{v+1} - t_v} \int_{t_v}^{t_{v+1}} \boldsymbol{p}(t)\, dt$.

Next we examine the optimization of the switching times. Consider a long experiment with a duration T and assume that the total number of switching events is fixed to the number N(T), presumably due to time and cost constraints. The loss function (with the Lagrange multiplier) is given by,

$$L(\mathrm{N(T)}, \mathrm{T}) = \sum_{v=0}^{N(T)-1} \int_{t_v}^{t_{v+1}} \sum_{ij} p_{i|j}(t) p_j^s \log\left(\frac{p_{i|j}(t)}{\sum_k W_{ik}^{-1} b_{k|j}(t)}\right) dt - \lambda\left(\sum_k b_{k|j} - 1\right).$$

We now ask at what times it is best to switch? To answer, we take the derivative with respect to the switching time(s),

$$\frac{\partial}{\partial t_k} L(\mathrm{N(T)}, \mathrm{T}) = \sum_{v=0}^{N(T)-1} \frac{\partial}{\partial t_k} \int_{t_v}^{t_{v+1}} \sum_{ij} p_{i|j}(t) p_j^s \log\left(\frac{p_{i|j}(t)}{\sum_k W_{ik}^{-1} b_{k|j}(t)}\right) dt = 0$$

$$\Rightarrow 0 = \sum_{ij} p_{i|j}(t) p_j^s \log\left(\frac{p_{i|j}(t)}{\sum_k W_{ik}^{-1} b_{k|j}(t)}\right)\Bigg|_{t_{k-1}}^{t_k} - \sum_{ij} p_{i|j}(t) p_j^s \log\left(\frac{p_{i|j}(t)}{\sum_k W_{ik}^{-1} b_{k|j}(t)}\right)\Bigg|_{t_k}^{t_{k+1}}$$

$$\sum_{ij} p_{i|j}(t_k) p_j^s \log\left(\frac{p_{i|j}(t_k)}{\sum_k W_{ik}^{-1} b_{k|j}(t_k)}\right) - \sum_{ij} p_{i|j}(t_{k-1}) p_j^s \log\left(\frac{p_{i|j}(t_{k-1})}{\sum_k W_{ik}^{-1} b_{k|j}(t_{k-1})}\right) =$$

$$\sum_{ij} p_{i|j}(t_{k+1}) p_j^s \log\left(\frac{p_{i|j}(t_{k+1})}{\sum_k W_{ik}^{-1} b_{k|j}(t_{k+1})}\right) - \sum_{ij} p_{i|j}(t_k) p_j^s \log\left(\frac{p_{i|j}(t_k)}{\sum_k W_{ik}^{-1} b_{k|j}(t_k)}\right)$$

This has a simple interpretation that for a given responsive strategy the optimal switching times should be distributed to allow for equal loss between consecutive switching events.

## (V) Generalized growth matrix for the case of n independent uptake/de-novo synthesis decisions

In the paper we presented an experiment that poses a binary dilemma to cells. In this environment, cells can choose either to import an amino acid or alternatively to synthesize it from more elementary nutrients present in the environment. Here we generalize this example further to the case of $n$ independent such choices. There are two interesting aspects to this generalization. First, the obtained growth rate per environment matrix (the $O$ matrix) turns out to be orthogonal, and second, it serves as a starting point to a more general theory regarding correlated choices i.e. when the choice of substrate affects other choices, due to biochemical constraints. These correlations effectively reduce the dimensionality of the strategy space.

First let us define "catabolic end-product" (CEP). We define a CEP to be a material that is produced by the cell in a minimal environment as a precursor to essential elements such as protein, RNA, DNA or membrane synthesis. In other words, a CEP is an essential precursor that the cell internally produces in a minimal environment and there can be no growth without it.

Among the CEPs there is a subset that can be imported from the external environment. Most notably, amino-acids, deoxyribonucleosides such as thymine, NADH and several vitamins such as $B_{12}$. If a certain CEP is missing from the environment, the cell has to produce in order to maintain growth. However in the presence of a CEP in the environment, the cell can import it while reducing the internal production rate or alternatively, the cell can continue to produce it without importing. The cell can also do anything in between e.g. maintain a basal level of production while mostly importing, partially shut-down production, or relay solely on importing while closing internal production completely.

Consider again a minimal environment supplemented with $n$ such CEP's. Then for each CEP there are two extreme phenotypes namely (i) internal production of the CEP. (ii) optimal mixture of internal production and import (the optimal mixture can either be $100\%$ import or a

mix of import and internal production with a nonzero weight on import. These extreme phenotypes are convexly dominating the entire strategy space, as any policy can be written as a convex sum of the extreme policies.

If we allow only two possibilities per CEP i.e. either it exist in a *fixed concentration* or it is absent from the environment, then there are $2^n$ possible combinations of environments starting from a minimal environment with no external CEP's (M9 medium) to an environment with $k$ out of n CEPs supplemented to the minimal environment.

There are also $2^n$ extreme phenotypes, where a representative extreme phenotype is producing $k'$ CEP's internally and tries to import the rest (possibly moderately). The growth rate per environment matrix is not symmetric since the consequence of trying to import a CEP that is missing from the environment is a very harmful strategy while continuing the internal production of a CEP even though it is present in the environment might be suboptimal but not harmful.

We can represent the environments by a binary vector of length $n$ with the minimal media represented by the null vector and the media with all $n$ CEPs supplemented by the all ones vector. The media with (say) the $l^{\text{th}}$ CEP supplemented will be represented by a vector which is one in the $l$ component.

Similarly, we can represent the extreme phenotypes the same way only now a zero in the $l^{\text{th}}$ element represents a phenotype that chooses to internally produce the $l^{\text{th}}$ CEP while a one represent the attempt to import this CEP (reflected e.g. by the expression of transporters suitable for this CEP).

I the next figure, we present the global structure of the growth rate of each phenotype per environment for n=6 CEP's. In blue we mark positive growth (larger than one) and in white we mark negative growth (less than one). If we replace any nonzero element in the matrix by one, this matrix is also orthogonal.

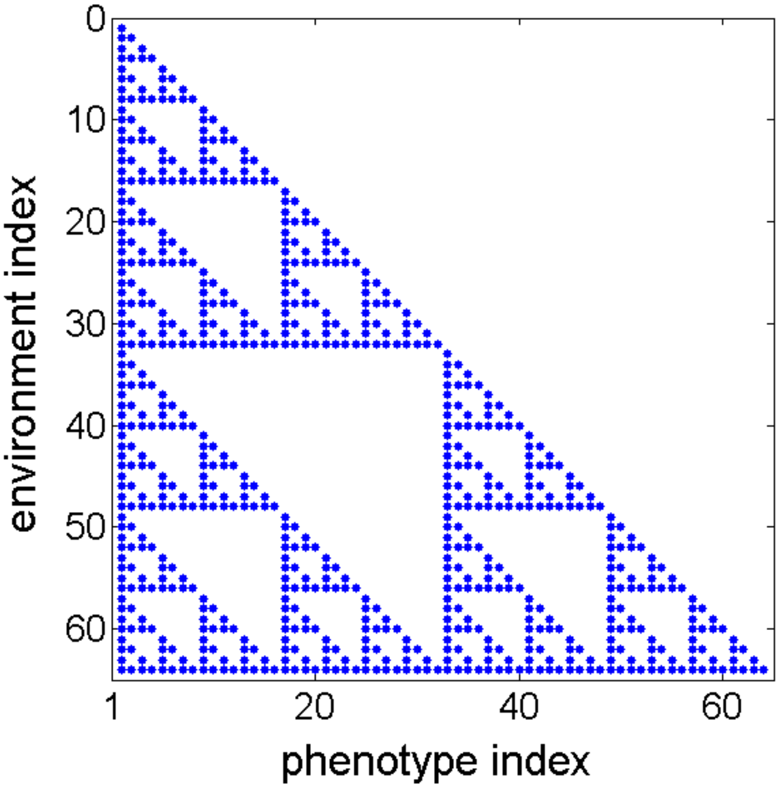


Figure S3: structure of the non-diagonal growth matrix $O$ for the n=6 binary choices game. The size of the matrix is $64 \times 64$. Blue dots represent non-zero elements. Interestingly, the inverse matrix is given by $O_{ij}^{-1} = \frac{1}{O_{ji}}$.

Case of multiple carbon sources

Consider the case where there are $n$ different carbon sources in the external environment. The cell can decide to uptake anything between one to all of the carbon sources. Assume that the each of the carbon sources is either present in abundance or absent. Then the number of possible environments is $2^n$. Since we want to study growth rather than quiescence, we erase the environment with no carbon sources so the total number of of environments is $2^n - 1$. In general, if we consider $m$ possible concentration levels for each carbon source, the dimensionality increases to $m^n - 1$.

In response to these environments, the cell can utilize particular metabolic pathways for import and processing of the carbon source available. For each of the carbon source types the cell can either utilize it or not. Therefore the number of possible combination is also $2^n - 1$. The global structure of the growth matrix is determined by the condition that the only non viable cells are

cells that attempt to utilize exactly the carbon sources that are missing from the environment. The resulting non diagonal matrix has an anti-diagonal form (where blue marks the positive growth and white the negative ones).

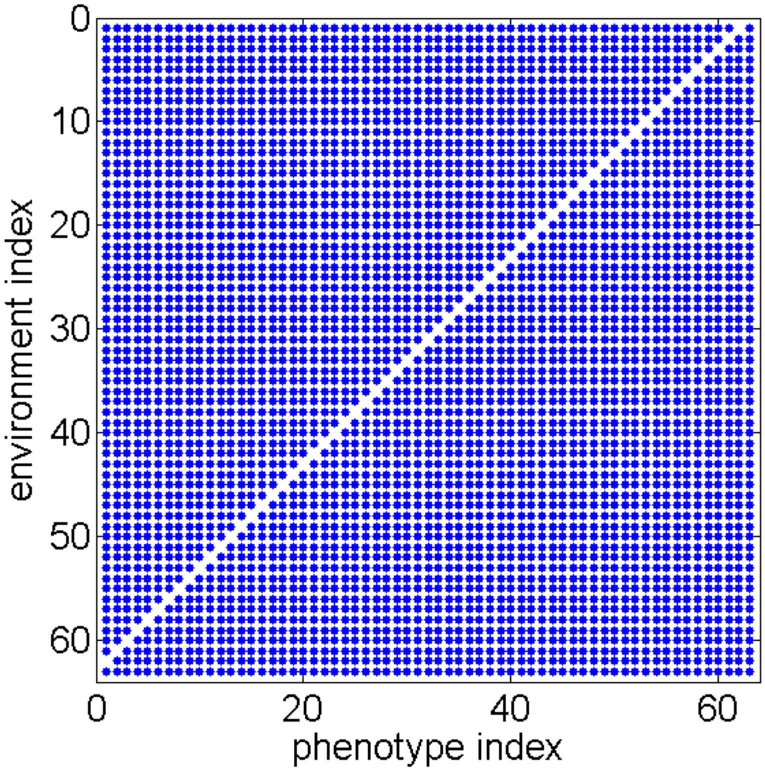


To summarize, by carefully considering all possible viable configuration of environments posing a choice dilemma for the cells we can construct different realizations of the growth matrix structure.

<u>An illuminating example</u>

As a final example, we consider the phenomenon of chromatic adaptation (see [A3] and references therein). Recent discoveries revealed that certain photosynthetic cyanobacteria striving in the ocean can modify their light harvesting antennas to allow better absorption of light required for growth. As cyanobacteria sinks, the ambient light level is attenuated and blue shifted compared to the level at zero depth.

Below a certain depth, there is not enough light to sustain growth. It is known that cyanobacteria can modulate the number of light harvesting antenna as a function of the ambient light intensity. Chromatic adaptation is even more spectacular, as it reveals a change in the absorption spectrum caused by a change in the types of light harvesting antenna expressed. This modification is light sensitive; it appears that a small light sensitive protein network

modulates the expression of different light harvesting antenna types that differ by the position of their absorption peaks as a function of the ambient wavelength. As the bacteria sinks, the light level becomes blue shifted, and the bacteria respond by changing the type of antenna to an antenna type that absorbs more light that is blue shifted, thus mitigating the change in the ambient spectrum and vice-versa, as currents lift the bacteria back to shallower waters, the expression profile switches back to antenna types that better absorb around yellow.

This system is particularly interesting for testing our model since the measurement of the environment; the side information and the information utilization are all spectral and hence rather accessible and visual. To be more concrete, consider an experiment where cyanobacteria capable of chromatic adaptation are placed in a constantly replenished chemical medium at fix temperature lacking organic carbon sources but containing dissolved $CO_2$. The medium is illuminated with a constant intensity but with varying spectrum. Experimentally, this can be achieved by changing a window in front of a wide-band lamp that is stabilized to yield constant intensity.

By measuring the absorption spectra of the cyanobacteria and by observing their color (the photosensitive protein sensors are visible to the naked eye, see [A3] and references therein) it is possible to estimate the population level information utilization rate and side information.

## (VI) The essential part of the game

To reduce any growth matrix to its essential form, one has to calculate the solution to the game, as defined by the growth matrix, and then eliminate from it the rows and columns that correspond to zeroes in the solution vectors. The idea behind this elimination is simple. If a strategy is not recommended by the game-theoretic solution, it means that it is always possible to gain more by avoiding it. Thus, we can eliminate it from the game altogether.

Below, a short Matlab code that returns the game-theoretical optimal strategy for the cell (`bgame`), nature (`pgame`), the game value, (`v`) and the essential part of the game (`Messential`).

```
function [bgame,pgame,v,Messential]=SolveZeroSumMatrixGame(M,Tol)
%function[bgame,pgame,v,Messential]=SolveZeroSumMatrixGame(M,opt,c,Tol)
%returns the game theoretic Nash equilibrium bgame and pgame for the zero
%sum matrix game given by M, the game value, v and the essential part of
%the game Messential.

sz=size(M);
[p,v1]=linprog(-[1;zeros(sz(1),1)],[ones(sz(2),1) -M'],...
    zeros(sz(2),1),[0 ones(1,sz(1))],1,[-inf;zeros(sz(1),1)]);
[b,v2]=linprog([1;zeros(sz(2),1)],[-ones(sz(1),1) M],...
    zeros(sz(1),1),[0 ones(1,sz(2))],1,[-inf;zeros(sz(2),1)]);
bgame=b(2:end);
pgame=p(2:end);
v=(pgame(:))'*M*bgame(:);
if nargin==1
  Tol=1e-5;
end
ib0=find(bgame<Tol);
ip0=find(pgame<Tol);
Messential=M;
Messential(:,ib0)=[];
Messential(ip0,:)=[];
```

## Bibliography

[A1] Ping Wang, Lydia Robert, James Pelletier, Wei Lien Dang, Francois Taddei, Andrew Wright, Suckjoon Jun, Current Biology, 22 June 2010 (Vol. 20, Issue 12, pp. 1099-1103).

[A2] Yu Liu, Biochemical Engineering, 25 april 2006 (Journal 31, pp. 102-105).

[A3] David M. Kehoe, PNAS, May 18, 2010. Vol. 107, p. 9029.
